# Supplementary material for: Exploring the limits of decoder-only models trained on public speech recognition corpora
Source: arXiv:2402.00235 source file (2024-01-31)
Supplement: Supplementary file 1 [file supplemental.tex]

\appendix

\section{Supplemental Material}\label{sec:supplemental}

\subsection{Additional Experiments}\label{sec:additional}

\subsection{Experimental Setup}\label{sec:experimental-setup}

In this section, we describe the training details for the experiments presented in \S\ref{sec:experiments}.

\paragraph{Details for Table \ref{tab:shift}} Same as details for Table \ref{tab:atomic-tasks} except $H = 32$, batch size is 4, number of layers is 1 and number of steps was $86K$. Learning rate was 1e-5 for \dlr. $\alpha$-min and $\alpha$-max were 1e-5 for \textsc{SGConv} to avoid signal decay, kernel dimension $d=4096$ and number of concatenated kernels (i.e. number of scales) was computed so that the resulting kernel is at least as long as the input. The kernel parameters were initialized from $\mathcal{N}(0,\sigma^2=d^{-2})$.

Experiments in Table \ref{tab:atomic-tasks} and \ref{tab:shift} were performed on a single NVIDIA 3090 (24GiB).

\begin{table*}[h]
  \centering
  \small
%   \resizebox{\textwidth}{!}{%
    \begin{tabular}{@{}llllllllllll@{}}
      \toprule
                                      & L & layers & H & N & dt-min & dt-max & LR & Batch Size & steps & epochs  \\
      \midrule
      \dlr      &   $2^{12}$       & 1 / 6             & $2^{7}$                       & $2^{12}$            & 1e-5             & 1e-5     & 1e-4     & 16              & $40K$           & 12                 \\
     \dssexp      &   $2^{12}$       & 1              & $2^{7}$                       & $2^{12}$            & 1e-4             & 1e-2     & 1e-3     & 16              & $40K$           & 12                 \\
    \attention     &   $2^{12}$       & 1              & $2^{7}$                       &             &               &       & 1e-3     & 16              & $40K$           & 12                 \\
    \dlr      &   $2^{9}$       &  6             & $2^{7}$                       & $2^{12}$            & 1e-5             & 1e-5     & 5e-5     & 64              & $11K$           & 12                 \\
    \attention     &   $2^{9}$       & 2              & $2^{7}$                       &             &               &       & 1e-3     & 64              & $11K$           & 12                 \\
    \bottomrule
    \end{tabular}%
%   }
  \caption{
    Hyperparameters for Table \ref{tab:atomic-tasks} on all tasks except \textsc{MIPS}. Exceptions are detailed in \S\ref{sec:experimental-setup}. LR is initial learning rate.
  }\label{tab:atomic-hyperparams}
\end{table*}
